# Supplementary material for: Learning Causal Response Representations through Direct Effect Analysis
Source: arXiv:2503.04358 source file (2025-03-06)
Supplement: Supplementary file 1 [file supp.tex]

\clearpage
\newpage

\section{Robustness of common multivariate analysis algorithm}\label{sec:robustness_common_MVA}
In this section, we aim to prove the compatibility and incompatibility of some standard multivariate analysis algorithms. 
We assume that the $(X, Y, H, A)$ distribution be entailed in Eq.~\eqref{Eq:anchor-model}.

A natural extension of Ordinary Least Squares ($\ell_2$) regression to the multioutput case is to solve an OLS problem for each output, which is equivalent to solving the optimisation problem:
\begin{align}
    \min_{\mathbf{W} \in \mathbb{R}^{d\times p}} \mathbb{E}\|Y - \mathbf{W}^TX\|_F^2,
\end{align}
also known as multilinear (or multioutput) regression. Extra constraints on the regression coefficients can be added, leading, for example, to Reduced Rank Regression by constraining $\mathbf{W}$ to be of rank $\rho < \min(p, d)$. This constraint resembles constraining $\mathbf{W}$ to have the form $\mathbf{V}^T\mathbf{U}$, with $\mathbf{U} \in \mathbb{R}^{\rho\times d}$ and $\mathbf{V}\in \mathbb{R}^{\rho\times p}$.

This formulation is closely related to the formulation of Orthogonalised Partial Least Squares with an extra constraint on the ordering of the columns of $\mathbf{V}^TX$ based on their predictive performance on $Y$. Therefore, we derive the proof of anchor compatibility for the multilinear regression setting, which directly extends to anchor compatibility of OPLS and Reduced Rank Regression.

Since both OPLS and RRR aim to achieve the same objective as defined in Eq.~\eqref{Eq:OPLS_RRR} with different constraints on regression coefficients $\mathbf{W}$, we prove the general anchor compatibility of MLR, but this extends to OPLS and RRR.

\begin{proposition}[Multilinear, Reduced Rank and Orthonormalised Partial Least Square Regression are \emph{anchor-compatible}.]
    The algorithm minimising the expectation of the following loss function:
    \begin{align}\label{Eq:OPLS_RRR}
        \mathcal{L}(X, Y; \mathbf{\Theta}) = \|Y - \mathbf{W}^TX\|^2_F
    \end{align}
    is \emph{anchor-compatible}. Here $\|.\|_F$ defines the Froebinius norm.
\end{proposition}

\begin{proof}
The proof of this proposition is straightforward, observing that the loss can be written as:
\begin{align}
    \mathcal{L}(X, Y; \mathbf{\Theta}) = \sigma_Y - \mathbf{W}^T\sigma_{XY} + \mathbf{W}^T\sigma_{X}\mathbf{W},
\end{align}
which is linear over the variance-covariance $\Sigma_{XY}$.

\end{proof}

Another type of Multivariate Analysis algorithm is not aimed at minimising prediction error. Instead, it focuses on maximising the similarity between latent representations of the predictors $X\mathbf{W}_x$ and the target $Y\mathbf{W}_y$. A standard measure of this similarity is covariance, leading directly to the Partial Least Squares (PLS) algorithm, for which we now present anchor compatibility.

\begin{proposition}[Partial Least Square regression is \emph{anchor-compatible}.]\label{prop:ac_pls}
    The PLS Regression algorithm maximising the expectation of the following loss function is \emph{anchor-compatible}:
    \begin{align}\label{Eq:PLS_loss}
        \mathcal{L}(X, Y; \mathbf{W}) = \frac{\text{tr}(\mathbf{W_x}^TC_{XY}\mathbf{W}_y)}{\sqrt{\text{tr}(\mathbf{W_x}^T\mathbf{W_x})}\sqrt{\text{tr}(\mathbf{W_y}^T\mathbf{W_y})}}.
    \end{align}
     
\end{proposition}

\begin{proof}
The loss function Eq.~\ref{Eq:PLS_loss} is clearly linear with respect to the variance-covariance $\Sigma_{XY}$, which is sufficient to ensure the anchor compatibility of PLS regression.
\end{proof}

On the other hand, one could consider correlation as a measure of the similarity between the learned latent spaces, aiming to account for potential differences in the variance of each variable and thus assigning equal weight to each dimension of the latent space. This approach is generally known as Canonical Correlation Analysis (CCA) or PLS mode B. By considering the variance of the latent representation of the predictors and the target, we sacrifice linearity with respect to the variance-covariance of $X$ and $Y$ (as illustrated in Eq.~\ref{Eq:CCA_loss}), making CCA incompatible with anchor regularisation.

\begin{example}[Canonical Correlation Analysis is not \emph{anchor-compatible}.]\label{ex:incompatibility_CCA}
    The Canonical Correlation Analysis solving the optimisation problem 
    \begin{align}\label{Eq:CCA_loss}
        \mathcal{L}(X; \mathbf{W}) = \frac{\text{tr}(\mathbf{W_x}^T\Sigma_{XY}\mathbf{W_y})}{\sqrt{\text{tr}(\mathbf{W_x}^T\Sigma_{X}\mathbf{W_x})} \sqrt{\text{tr}(\mathbf{W_y}^T\Sigma_{Y}\mathbf{W_y})}}
    \end{align}
    is not \emph{anchor-compatible} as it is not linear over the variance-covariance matrix. This explains the different behaviour taken by anchor regularisation in Fig.~\ref{fig:perturbation_strength} by the anchor-regularised CCA.
\end{example}

This is illustrated in Fig.~\ref{fig:perturbation_strength}, where we can observe that anchor-regularised CCA exhibits a distinct behavior compared to anchor-compatible MVA algorithms. It would be of interest to investigate to which extent the incompatibility of CCA with anchor regularisation impacts its distributional robustness properties and if its anchor regularisation could still be of interest.

\paragraph{OPLS formulations and their relation to CCA}\label{par:CCA_OPLS_eq}
There are two versions of OPLS: the standard eigenvalue decomposition (EVD) and the generalized eigenvalue (GEV) formulations~\cite{Arenas-Garcia1015}. In our work, we implement EVD-OPLS whose optimization problem is 
\begin{align*}
\min_{\mathbf{U},\mathbf{V}} & \| Y - \mathbf{U} \mathbf{V}^T X\|_F^2\\
&\text{s.t. } \ \mathbf{U}^T\mathbf{U} = \mathbf{I}.
\end{align*}
EVD-OPLS is linear in $C_{XY}$ and is, therefore, an anchor-compatible loss. On the other hand, the GEV-OPLS loss is 
\begin{align*}
\min_{\mathbf{U},\mathbf{V}} & \| Y - \mathbf{U} \mathbf{V}^T X\|_F^2\\
&\text{s.t. } \ \mathbf{V}^TC_X\mathbf{V} = \mathbf{I} 
\end{align*}
Viewing the optimization for $\mathbf{V}$ as a generalized eigenvalue decomposition problem by absorbing the constraint into the loss gives us the equivalent optimization 
\begin{equation*}
    \min_{\mathbf{v}} \frac{\mathbf{v}^T X^T Y Y^T X \mathbf{v}}{\mathbf{v}^T C_X \mathbf{v}}.
\end{equation*}
This is clearly \emph{not} linear in $C_{XY}$ because it is not linear in $C_{X} = X^TX$.

Furthermore, GEV-OPLS and CCA are shown to be equivalent up to an orthogonal rotation \citep[see][Theorem 2]{Sun2009}, and by similar reasoning, CCA is also not anchor-compatible. 

\section{Proofs}

\subsection{Proof of Theorem~\ref{thm:ACloss}}
\begin{proof}
    Let's first note that from the SCM Eq.~ \ref{Eq:anchor-model} we have the following decomposition:
    \begin{align*}
        f(C_{X Y}) &= f(\mathbf{D}C_\varepsilon\mathbf{D}^T + \mathbf{D} \mathbf{M}C_A \mathbf{M}^T\mathbf{D}^T)\\
        &= f(\mathbf{D}C_\varepsilon\mathbf{D}^T) + f(\mathbf{D} \mathbf{M} C_A \mathbf{M}^T\mathbf{D}^T)
    \end{align*}
    by linearity of $f$. Thus when taking the supremum of the expectation of $f(C_{X Y})$ over $C^\gamma$, we get
    \begin{align*}
        \sup_{\nu \in C^\gamma} \Enu[f(C_{X Y})] &= f(\mathbf{D}\Sigma_\varepsilon\mathbf{D}^T) \\
        &+ \sup_{\nu \in C^\gamma} f(\mathbf{D} \mathbf{M} \Sigma_\nu \mathbf{M}^T\mathbf{D}^T),
    \end{align*}
    %as the left term 
    since $f(\mathbf{D}\Sigma_\varepsilon\mathbf{D}^T)$ is not affected by the intervention. Using the definition of $C^\gamma$ leads to 
    \begin{align}
    \begin{split}
\label{Eq:loss_decomp_final}
        \sup_{\nu \in C^\gamma} \Enu[f(C_{X Y})] &= f(\mathbf{D}\Sigma_\varepsilon\mathbf{D}^T) \\
        &+ \gamma f(\mathbf{D} \mathbf{M} \Sigma_A \mathbf{M}^T\mathbf{D}^T).
        \end{split}
    \end{align}
    Let's now note that for $(A, X, Y) \sim \mathbb{P}_{\text{train}}$ we have
    \begin{align*}
        \Etrain \left [\begin{pmatrix}X \\ Y\end{pmatrix} | A \right] &= \mathbf{D} \Etrain[\varepsilon|A] + \mathbf{D} \mathbf{M}\Etrain[A|A] \\
        &=  \mathbf{D}\mathbf{M}A,
    \end{align*}
    where $\mathbb{P}_{\text{train}}$ is the training distribution.

    As $\varepsilon$ is mean centred and independent of $A$. Thus, we can write 
    \begin{align*}
        f(C_{X Y|A}) = f(\mathbf{D}\mathbf{M}C_A\mathbf{M}^T\mathbf{D}^T)
    \end{align*}
    by linearity of $f$. Taking its expectation over the training distribution, we get
    \begin{align}
\label{Eq:Decomp_right_term}
        \Etrain[f(C_{X Y| A }) ] = f(\mathbf{D}\mathbf{M}\Sigma_A\mathbf{M}^T\mathbf{D}^T),
    \end{align}
    which is similar to the right term of Eq.~\eqref{Eq:loss_decomp_final} as $\Etrain[f(C_{X Y| A }) ]= f(\Sigma_{X Y| A })$. A similar reasoning leads to 
    \begin{align}\label{Eq:Decomp_left_term}
      \Etrain[ f(C_{X Y})] -  \Etrain[f(C_{X Y|A})] &= f(\mathbf{D}\Sigma_\varepsilon\mathbf{D}^T).
    \end{align}
    
    Pluging-in Eq.~\eqref{Eq:Decomp_right_term} and Eq.~\eqref{Eq:Decomp_left_term} in Eq.~\eqref{Eq:loss_decomp_final} we get
    \begin{align*}
        \sup_{\nu \in C^\gamma} &\Enu[f(C_{X Y})] = \\
         &\Etrain[ f(C_{X Y})]  + (\gamma-1) \Etrain [f(C_{X Y|A}) ]\\
       = &f(\Sigma_{X Y}) + (\gamma-1)  f(\Sigma_{X Y|A}),
    \end{align*}
    which concludes the proof.
\end{proof}

\subsection{Proof of Equivalence for Transformed Data}

\begin{proof}
\label{pr:proof_estimator}
From 
\begin{align}\label{Eq:perturbed_data}
    \begin{split}
        \tilde{\mathbf{X}} &= (\mathbf{I} + (\sqrt{\gamma} - 1)\Pi_\mathbf{A}) \mathbf{X}\\
        \tilde{\mathbf{Y}} &= (\mathbf{I} + (\sqrt{\gamma} - 1)\Pi_\mathbf{A}) \mathbf{Y},
    \end{split}
\end{align}
 we can easily derive that 
 \begin{align*}
     \mathbf{S}_{\tilde{X}\tilde{Y}} = & \frac{1}{n-1} (\tilde{\mathbf{X}}\tilde{\mathbf{Y}})^T (\tilde{\mathbf{X}}\tilde{\mathbf{Y}})\\
     = &\frac{1}{n-1} ((\mathbf{X}\mathbf{Y} + (\sqrt{\gamma} - 1)\Pi_\mathbf{A}\mathbf{X}\mathbf{Y})^T \\
      &(\mathbf{X}\mathbf{Y} + (\sqrt{\gamma} - 1)\Pi_\mathbf{A} \mathbf{X}\mathbf{Y}))\\
\end{align*}
As $\Pi_\mathbf{A}$ is an orthogonal projection, we have that $(\mathbf{X}\mathbf{Y})^T  (\Pi_\mathbf{A} \mathbf{X}\mathbf{Y}) = \Pi_\mathbf{A} (\mathbf{X}\mathbf{Y})^T\mathbf{X}\mathbf{Y} = \mathbf{S}_{XY|A}$, leading to
\begin{align*}
      = & \mathbf{S}_{XY} + 2(\sqrt{\gamma}-1)\mathbf{S}_{XY|A}\\
      + &(\sqrt{\gamma}-1)^2\mathbf{S}_{XY|A}\\
      = &\mathbf{S}_{XY} + (\gamma-1)\mathbf{S}_{XY|A}.
 \end{align*}
Thus, we have that $\argmin_{\mathbf{\Theta}} f_{\mathbf{\Theta}}(\mathbf{S}_{\tilde{X}\tilde{Y}})$ is
 \begin{equation*}
      \argmin_{\mathbf{\Theta}} f_{\mathbf{\Theta}}(\mathbf{S}_{XY}) + (\gamma-1) f_{\mathbf{\Theta}}(\mathbf{S}_{XY|A})
 \end{equation*}
by linearity of $f_{\mathbf{\Theta}}$ which concludes the proof.
\end{proof}

\section{Details for the Simulation Experiments}
\subsection{Experiment setting}\label{par:toy_experimental_setting}

The results of the simulation experiments are obtained as follows. The training data are sampled following Eq.~\eqref{Eq:toy_model_IV}, and the testing data are generated by modifying $\varepsilon_A$ such that $\varepsilon_A\sim \mathcal{N}(0, t)$. The perturbation strength $t$ is varied over a linear sequence $t\in [0, 4]$ with $20$ steps. 
We repeat each experiment $B=10$ times by sampling $n=300$ training and testing samples of $(A, X, Y)$.
We plot the average Mean Squared Errors in Fig.~\ref{fig:perturbation_strength} and Fig.~\ref{fig:perturbation_strength_non_gaussian_noise}. Both $A$ and $H$ are one-dimensional, while $X$ and $Y$ are $10$-dimensional. The matrix $\mathbf{W}$ is generated as a low-rank (of rank $\rho$) matrix such that $\mathbf{W} = \mathbf{U}\mathbf{V}$ with $\mathbf{A}\in \mathbb{R}^{d\times \rho}$ and $\mathbf{B}\in \mathbb{R}^{\rho\times p}$. The coefficients of $\mathbf{A}$ and $\mathbf{B}$ are sampled uniformly between $1$ and $2$ and are normalised such that their sum is $1$.

The algorithm CCA, PLS, and MLR come from the \emph{scikit-learn} library (respectively CCA, PLSRegression and LinearRegression learners). We use the code provided with the paper \cite{Mukherjee2011} available at \href{https://github.com/rockNroll87q/RRRR}{https://github.com/rockNroll87q/RRRR} for the Reduce Rank Regression algorithm and our implementation of OPLS based on \cite{Arenas-Garcia1015} using an eigenvalue decomposition as we use the constraint $A^TA=\mathbf{I}$.

\paragraph{High-dimensional setting} We also conduct a high-dimensional experiment to evaluate the performance of anchor-regularized algorithms when the dimensionality of $X$ and $Y$ exceeds the sample size. We generate data by sampling $n=200$ instances of $X$ and $Y$, each with a dimensionality of $d=p=300$. The rank of $\mathbf{W}$ is set to $\rho = 100$. We compare the results between Ridge Regression and Reduced Rank Ridge Regression. As shown in Figure \ref{fig:perturbation_strength_high_dim}, both methods demonstrate robustness across a wide range of perturbation strengths.

\begin{figure}
    \centering
    \includegraphics[width=0.45\textwidth]{figures/perturbation_robustness_IV_high_dim.pdf}
    \caption{Experiments in high-dimensional setting with $d=p=300$ and $n=200$. We can see that both Multi-output Ridge Regression and Reduced rank Ridge Regression are optimal for a wide range of perturbation strength. }
    \label{fig:perturbation_strength_high_dim}
\end{figure}

\paragraph{Non-gaussian noise experiments}
To assess the robustness of our results presented in paragraph \ref{Par:Toy_model_results}, we conducted the same toy model experiments with noise $\varepsilon_A$, $\varepsilon_H$, $\varepsilon_X$, and $\varepsilon_Y$ following an exponential distribution (Fig.~\ref{fig:perturbation_strength_non_gaussian_noise}.A) and a gamma distribution (Fig.~\ref{fig:perturbation_strength_non_gaussian_noise}.B) with scales $1$.

As observed in Fig.~\ref{fig:perturbation_strength_non_gaussian_noise}, anchor-regularised models remain optimal for a wide range of perturbation strengths, except for anchor-regularised CCA. The behavior of anchor-regularised CCA is explained by its incompatibility with anchor regularisation.

\begin{figure*}[t]
    \centering
    \includegraphics[width=0.9\textwidth]{figures/perturbation_strength_robustness_IV_exponential_noise.pdf}

    \includegraphics[width=0.9\textwidth]{figures/perturbation_strength_robustness_IV_poisson_noise.pdf}

    \includegraphics[width=0.9\textwidth]{figures/perturbation_strength_robustness_IV_uniform_noise.pdf}
    \caption{Similar experiments as in \ref{Par:Toy_model_results} with noise sampled from non-gaussian distributions. (Top) Exponential distribution of scale$1$, (Middle) Poisson distribution of parameter $1$, (Bottom) Uniform distribution between $-2$ and $2$. We see that all the \emph{anchor-compatible} algorithms are robust to increasing perturbation strength. }
    \label{fig:perturbation_strength_non_gaussian_noise}
\end{figure*}

\begin{figure*}[t]
    \centering
    \includegraphics[width=0.9\textwidth]{figures/perturbation_strength_robustness_IV_fig3Anchorpaper.pdf}
    \caption{Experiment for anchor confounding $X$ and $Y$. We can see that all algorithms present a very robust behavior to increasing perturbation strength (even CCA which is not \emph{anchor-compatible}).}
    \label{fig:fig3_anchor_paper}
\end{figure*}

\paragraph{Confounding anchor experiment}\label{sec:confounding_experiment}

We also reproduced experiments from equation 12 in \cite{Rothenhäusler2018} to demonstrate how anchor-regularised MVA algorithms exhibit interesting robustness properties when the anchor has a confounding effect. These results are illustrated in Fig.~\ref{fig:fig3_anchor_paper}. Here, the training distribution is encapsulated in the following Structural Causal Model (SCM):
\begin{align}
    \begin{split}
        \varepsilon_A,\, \varepsilon_H,\, &\varepsilon_X,\, \varepsilon_Y \sim \mathcal{N}(0, 1),\\
        A &\leftarrow \varepsilon_A,\\
        H &\leftarrow A + \varepsilon_H,\\
        X &\leftarrow A + H + \varepsilon_X,\\
        Y &\leftarrow \mathbf{W}^TX + H + \varepsilon_Y,
    \end{split}
\end{align}

with again testing distribution sampled by setting $\varepsilon_A \sim \mathcal{N}(0, t)$ where $t$ is the perturbation strength and $\mathbf{W}$ being lower rank.

We can see that all algorithms exhibit robustness properties for a very large range of perturbation strength. It is interesting to note that CCA presents a similar behavior as the \emph{anchor-compatible} algorithms. It would be interesting to investigate in which specific cases CCA gives robustness properties. 

\subsection{Hyperparameters selection experiment}\label{par:toy_high_dim_detail}

The results of the toy model experiments in the high-dimensional setting are obtained as follows. The training data are sampled following the DAG

\begin{align}
    \begin{split}
        \varepsilon_A,\, \varepsilon_H,\, &\varepsilon_X,\, \varepsilon_Y \sim \mathcal{N}(0, 1),\\
        A &\leftarrow \varepsilon_A,\\
        H &\leftarrow \varepsilon_H,\\
        X &\leftarrow \frac{1}{2}A + H + \varepsilon_X,\\
        Y &\leftarrow 2A + \mathbf{W}^TX + H + \varepsilon_Y,
    \end{split}
\end{align}

and the testing data are generated by modifying $\varepsilon_A$ such that $\varepsilon_A\sim \mathcal{N}(0, t)$. The perturbation strength $t$ is set to $2$. We repeat each experiment $B=10$ times by resampling $n=100$ training and validation samples and $n=400$ testing samples of $(A, X, Y)$. Both $A$ and $H$ are one-dimensional, while $X$ and $Y$ are $300$-dimensional. The matrix $\mathbf{W}$ is generated as a low-rank (of rank $\rho$ which is randomly sampled uniformly on $[10, 30]$) matrix such that $\mathbf{W} = \mathbf{U}\mathbf{V}$ with $\mathbf{U}\in \mathbb{R}^{d\times \rho}$ and $\mathbf{V}\in \mathbb{R}^{\rho\times p}$. The coefficients of $\mathbf{U}$ and $\mathbf{V}$ are sampled uniformly between $1$ and $3$ and are normalised such that their sum is $1$. Hyperparameters $\alpha$ ranging from $1$ to $10^5$ are chosen from a logarithmic scale with $20$ candidates, while $\rho$ ranges from $10$ to $30$ linearly with $10$ candidates, and $\gamma$ ranges from $1$ to $10^4$ logarithmically with $10$ candidates. Performance, measured in terms of Mean Squared Error and Mean correlation between anchor variable and residuals, is evaluated on a validation set (not seen during training) and a perturbed testing set. We illustrate the results by selecting the optimal rank for each pair $(\gamma, \alpha)$ (see Figure \ref{fig:pareto-ARRRR}). Optimal parameters are chosen to minimize different objectives: for RRRR, parameters $(\alpha, \rho)$ that minimize training MSE are selected, while for A-RRRR, a convex combination of correlation between anchor and residuals ($g_1(\gamma, \alpha, \rho)$) and MSE ($g_2(\gamma, \alpha, \rho)$) at training is minimized, i.e., $(\gamma, \alpha, \rho) = \argmin \sum_{i=1}^2 w_i \frac{g_i(\gamma, \alpha, \rho)}{\eta_i}$, where $\eta_1$ and $\eta_2$ rescale the two objectives. In Figure \ref{fig:pareto-ARRRR}, we present the results for optimal RRRR and A-RRRR with weights $w_1=0.1$ and $w_2=0.9$, emphasizing independence of anchor and residuals.

\begin{figure*}[!ht]
    \centering
    \includegraphics[width=0.9\textwidth]{figures/DIV_GMT_TRAIN_TEST.pdf}
    \caption{DIV and global forced response for a "low-variability" model (CESM2) (A) and for a "high-variability" model (CNRM-CM6-1) (B).}
    \label{fig:DIV_GMT_TRAIN_TEST}
\end{figure*}

\newpage

\section{Details of real-world experiment}\label{sec:real_world_details}

\paragraph{Optimal fingerprint for detection of forced warming}

In D\&A studies, the optimal fingerprinting process involves several steps. Firstly, the response of the climate system to an external forcing is extracted using a statistical learning model to predict the forced climate response, denoted as $Y^{\text{forced}}_{\text{mod}}$. This is achieved by utilising spatial predictors from a gridded field of climate variables $X_{\text{mod}}$, following the regression equation:
\begin{align}
    Y_{\text{mod}}^{\text{forced}} = X_{\text{mod}}\beta + \beta_0 + \varepsilon.
\end{align}
Here, the spatial fingerprint is represented by the regression coefficient $(\beta, \beta_0)$.
Subsequently, a detection metric is obtained by projecting observations ($X_{\text{obs}}$) and unforced simulations ($X_{\text{cntl}}$) (known as control scenarios) onto the extracted fingerprint $\hat{\beta}$. Practically, as multiple members and models are available for the unforced scenario, a distribution for $X_{\text{mod}}^{\text{cntl}} \hat{\beta} + \hat{\beta}_0$ can be obtained. Then, it is tested whether $X_{\text{obs}} \hat{\beta} + \hat{\beta}_0$ lies within the same distribution. If the test is rejected, a forced response is detected.

\paragraph{From Global to Regional}
Moving from a global to regional scale presents challenges in D\&A studies. One of the current challenges is transitioning from detecting a global forced response to a regional or local forced response. This is because climate variability magnitude is larger at regional scales, and even larger at a local scale, leading to a lower signal-to-noise ratio of the forced warming response. As the signal-to-noise ratio is in this case much lower, it becomes much more challenging to detect the forced signal. Additionally, different climate models and observations exhibit different patterns of internal variability at regional scales, necessitating the training of statistical learning models robust to potential distribution shifts in internal variability.

\paragraph{Robustness to multidecadal internal variability}

The ability to detect forced warming in Detection and Attribution studies is highly influenced by the level of internal variability \citep[see ][]{Parsons2020}. For instance, the observed 40-year Global Mean Temperature (GMT) trend of 0.76°C for the period $1980-2019$ would exceed the standard deviation of natural internal variability in CMIP5 and CMIP6 archive models classified as "low-variability" by a factor of $5$ or more \citep[see Fig. 1B in][]{Sippel2021}. However, for "high-variability" models, this trend exceeds the standard deviation only by a factor of $2$. This becomes evident when comparing models with "low-variability" (Figure \ref{fig:DIV_GMT_TRAIN_TEST} A) to those with "high-variability" (Figure \ref{fig:DIV_GMT_TRAIN_TEST} B), where it is less clear that internal variability alone could generate the Global Mean Temperature. This discrepancy poses a significant challenge, as in the former case, the observed warming has an extremely low probability of being generated by internal variability alone. Conversely, in the latter case, the rejection of the hypothesis that current temperature trends are solely attributable to internal variability is less robust.
For this reason, it is important to develop tests that are robust to changes in the magnitude of internal variability, particularly with the increasing magnitude of DIV. Assuming the DAG depicted in Figure \ref{fig:dag_DIV_Y_X}, anchor regularisation emerges as a suitable approach, enabling robust estimation robust to DIV increase.

\begin{figure}[t]
    \centering
    \begin{tikzpicture}[auto, scale=12,
    node distance = 18mm and 6mm,
    edge/.style ={arrows=-{Latex[length=3mm]}},
    dashededge/.style ={dashed}, % New style for dashed edges
    node/.style={circle,inner sep=1mm,minimum size=1cm,draw,black,very thick,text=black}]

     \node [node] (x) {$X$};
     \node [node] (y) [right of = x, xshift=12mm] {$Y^{\text{forced}}_{\text{mod}}$};
     %\node [node] (h) [above of = x, xshift=8mm]  {$H$};
     \node [node] (a) [left of = x, xshift=-12mm]  {$DIV$};

     %\path[edge] (a) edge (h);
     \path[edge] (a) edge (x);
     %\path[edge, bend left=12] (a) edge (y);

     %\path[edge, bend left=12] (h) edge (x);
     %\path[edge, bend left=12] (h) edge (y);

     \path[edge] (y) edge (x);
     \path[dashededge, bend right=20] (x) edge node[below] {$\mathbf{W}$} (y);
     %\path[edge, bend left=12] (x) edge (h);

     %\path[edge, bend left=12] (y) edge (x);
     %\path[edge, bend left=12] (y) edge (h);
     
    \end{tikzpicture}
    \caption{DAG considered for detection of forced warming response as proposed in \cite{Sippel2021}.}
    \label{fig:dag_DIV_Y_X}
\end{figure}

\paragraph{Climate models}
In this experiment, we utilised $7$ climate models from the CMIP5 and CMIP6 archives, each having at least $8$ members. The selection of these models was primarily practical, based on our access to them and their suitability for the train/test split procedure based on DIV magnitude.
\begin{table}[t]
    \centering
     % Adjust interline space
    \small
    \caption{Climate models used in this work, their number of members, associated DIV magnitude and corresponding set (train or test).}
    \begin{tabular}{lcccc}
        \toprule
        Model & CMIP   &  $\sharp$members & DIV mag. & Set \\
        \midrule
         {CCSM4} & 5   & 8 & 0.052 & Train \\
         {NorCMP1} & 6   &  30 & 0.064 & Train \\
         {CESM2} & 6   &  11 & 0.076 & Train \\
         {HadCM3} & 5   &  10 & 0.072 & Train \\
         {CNRM-CM6-1} & 6   &  30 & 0.175 & Test \\
         {CNRM-ESM2-1} & 6   &  10 & 0.174 & Test \\
         {IPSL-CM6A-LR} & 6   &  32 & 0.141 & Test \\
        \bottomrule
    \end{tabular}
    \label{tab:CMIP56_models}
\end{table}

\paragraph{Results}

\begin{table}[t]
    \centering
    \tiny
    \caption{Metrics for RRRR, and they anchor-regularised version with $\gamma=5$ and $\gamma=100$. We can see that both anchor-regularised approaches outperformed unregularised RRRR in term of $R^2$ score and mean correlation of residuals with DIV.}
    
    \begin{tabular}{lcccc}
        \toprule
         & \multicolumn{2}{c}{Test}    & \multicolumn{2}{c}{Train}  \\
         \cmidrule{2-3}\cmidrule{4-5}
          & $R^2$    & Mean correlation &   $R^2$    & Mean correlation  \\
        \midrule
         RRRR & 0.506 &  0.419 &  \textbf{0.510} &  0.157\\
        A-RRRR ($\gamma=5)$ & \textbf{0.537} &  0.248 & 0.500 &  0.120 \\
        A-RRRR ($\gamma=100)$& 0.533 &  \textbf{0.123} & 0.487 &  \textbf{0.096}\\
        \bottomrule
    \end{tabular}
    \label{tab:metrics_rrrr}
\end{table}
The anchor-regularised version of RRRR generally exhibits superior performance compared to its unregularised counterpart (refer to Table~\ref{tab:metrics_rrrr} and Figure~\ref{fig:corr_alpha}), both in terms of prediction performance (measured via $R^2$) and correlation between residuals and DIV at testing time. Notably, these results are achieved at a lower training time cost in terms of $R^2$, particularly when utilising $\gamma = 5$. This trade-off between performance during training and testing becomes clear when looking at the pareto front emerging (Figure ~\ref{fig:pareto_gamma_opt_CMIP56}) when considering different $\gamma$ values for optimal hyperparameters $(\alpha, \rho)$ selected via the validation procedure detailed earlier. We can see that selecting $\gamma$ such as it minimize an equally weighted ($\gamma 0.5/0.5)$ objectives (prediction performances and correlation between residuals and DIV) lead to a very small decrease during training but induce strong robustness (being close to optimal) at testing in terms of predicting performance.

Regarding the spatial patterns of prediction performance, anchor-regularised RRRR outperforms the unregularised version, particularly in the northern hemisphere and notably at the North Pole, where internal climate variability is significantly higher than closer to the equator. It also exhibits superior performance in northern regions where unregularised RRRR performs poorly, albeit with suboptimal results. Conversely, it demonstrates slightly better performance in the southern hemisphere, especially in regions where the DIV and the residuals exhibit anticorrelation (e.g., central Africa and the southern region of South America). In terms of the correlation between DIV and residuals, anchor-regularised RRRR outperforms the unregularised version across most regions, except for central Africa and the southern regions of South America, where residuals and DIV exhibit anticorrelation. On average, it reduces the correlation between residuals and DIV by more than $15\%$ for $\gamma=5$ and close to $30\%$ for $\gamma=100$.
\begin{figure}[!ht]
    \centering
    \includegraphics[width=0.40\textwidth]{figures/pareto_gamma_opt_30x60.pdf}
    \caption{Pareto front for A-RRRR with optimal $\alpha$, $\rho$, and $\gamma \in [1, 10^2]$ with optimal $\gamma$ of $0.5/0.5$ $0.1/0.9$ weighted objectives.}
    \label{fig:pareto_gamma_opt_CMIP56}
\end{figure}

\newpage

\begin{figure*}
    \centering
    \includegraphics[width=0.45\textwidth]{figures/R2_score_alpha.pdf}
    \includegraphics[width=0.45\textwidth]{figures/Correlation_score_alpha.pdf}
    \caption{(Left) $R^2$ scores (averaged uniformly). (Right) Mean correlation between DIV and residuals for different values of $\gamma$. }
    \label{fig:corr_alpha}
\end{figure*}

\newpage

\begin{figure*}
    \centering
    \includegraphics[width=0.8\textwidth]{figures/maps_anchor_R2_corr_30x60_gamma5.pdf}
    \label{fig:R2_corr_plot_gamma5}
    \caption{A-RRRR ($\gamma=5$) scores. (A)  $R^2$ scores. (B) Correlation between DIV and residuals.}
\end{figure*}

\begin{figure*}
    \centering
    \includegraphics[width=0.8\textwidth]{figures/maps_anchor_R2_corr_30x60_gamma100.pdf}
    \caption{A-RRRR ($\gamma=100$) scores. (A)  $R^2$ scores. (B) Correlation between DIV and residuals.}
    \label{fig:R2_corr_plot_gamma100}
\end{figure*}

\begin{figure*}
    \centering
    \includegraphics[width=0.8\textwidth]{figures/maps_rrrr_R2_corr_30x60.pdf}
    \caption{Unregularised RRRR scores. (A)  $R^2$ scores. (B) Correlation between DIV and residuals.}
    \label{fig:R2_corr_plot_rrrr}
\end{figure*}
